# Supplementary material for: Manifold Gradient Descent Solves Multi-Channel Sparse Blind Deconvolution Provably and Efficiently
Source: arXiv:1911.11167 source file (2021-04-06)
Supplement: Supplementary file 1 [file appendix_auxillary_details.tex]

\section{Auxiliary Details of Proof}

In this section, we provide more specific details used in the process of proof. The same notations introduced before are utilized.

\begin{lemma}\label{lemma:product_of_lipschitz}
    Fix any $\mathcal{D}\subseteq \mathbb{R}^n$, Let two functions $f_1,f_2: \mathcal{D}\rightarrow \mathbb{R}$. Assume $f_1$ is Lipschitz with $L_1$, $f_2$ is Lipschitz with $L_2$, and that $f_1, f_2$ are bounded over $\mathcal{D}$, i.e., for all $\bx\in \mathcal{D}$, $\abs{f_1(\bx)}\leq M_1$ and $\abs{f_2(\bx)}\leq M_2$ with $M_1,M_2>0$ are constants. Then the function $g(\bx)=f_1(\bx) f_2(\bx)$ is Lipschitz with $$L=M_1 L_2+ M_2 L_3.$$
\end{lemma}

\begin{proof}
    Fro any $\bx,\bx'\in \mathcal{D}$, we have
    \begin{equation}
        \begin{aligned}
        \abs{g(\bx)-g(\bx')}&=\abs{f_1(\bx) f_2(\bx)-f_1(\bx') f_2(\bx')}\\
        &\leq\abs{f_1(\bx) f_2(\bx)-f_1(\bx) f_2(\bx')}+\abs{f_1(\bx) f_2(\bx')-f_1(\bx') f_2(\bx')}\\
        &\leq M_1 L_2+ M_2 L_1
        \end{aligned}
    \end{equation}
\end{proof}

\begin{lemma} (Monotonically decreasing)\label{lemma:mono_dotpsi}
    Let $X\sim \mathcal{N}(0,\sigma_x^2), Y\sim \mathcal{N}(0,\sigma_y^2)$ and $\sigma_x\leq \sigma_y$, s.t we have
    \begin{equation}
        \mathbb{E}_{X}\sbra{1-\tanh^2(X)}\geq \mathbb{E}_{Y}\sbra{1-\tanh^2(Y)}
    \end{equation}
\end{lemma}

\begin{proof}
    Let $Z\sim \gd{1}$, as $1-\tanh^2(X)$ is monotoically decreasing with $\abs{x}$, we have
    \begin{equation}
    \mathbb{E}_{X}\sbra{1-\tanh^2(X)}=\int_Z \sbra{1-\tanh^2(\sigma_x Z)}dZ\geq \int_Z \sbra{1-\tanh^2(\sigma_y Z)}dZ= \mathbb{E}_{Y}\sbra{1-\tanh^2(Y)}
    \end{equation}
\end{proof}

\begin{lemma}\label{lemma:Operator norm of Circulant Matrix}
    Let $\bx\sim_{iid} BG(\theta)$ for $\theta\in(0,1]$. There exists some constant $C$, such that
    \begin{equation*}
        \mbP{\norm{\cC(\bx)} \geq t} \leq 2n \exp\sbra{\frac{-t^2}{C^2n}}, \quad \mbox{and}\quad        \mathbb{E}(\norm{\cC(\bx)}^{2m}) \leq \frac{m!}{2} \sbra{C n \log(n)}^m
    \end{equation*}
for all $m\geq 1$.
\end{lemma}

\begin{proof}
    As the operator norm of the circulant matrix $\norm{\cC(\bx)}$ is the maximum of the discrete fourier transform (DFT) of $\bx$, we turn to derive bound for DFT of $\bx$.

    Denoting the DFT of $\bx$ as $\lambda_k, k=1,\cdots n$, we are going to show that $\abs{\lambda_k}$ is sub-Gaussian with $\snorm{\abs{\lambda_k}}\leq C \sqrt{n}$ for some constant $C$. 
    
    First, by definition we have
     \begin{equation}
        \begin{aligned}
        \abs{\lambda_k}&=\sqrt{\sbra{\sum_{j=0}^{n-1}x_{j+1}\cos(\frac{ 2\pi jk}{n})}^2+\sbra{\sum_{j=0}^{n-1}x_{j+1}\sin(\frac{ 2\pi jk}{n})}^2}\\
        &\leq \abs{\sum_{j=0}^{n-1}x_{j+1}\cos(\frac{ 2\pi jk}{n})}+ \abs{\sum_{j=0}^{n-1}x_{j+1}\sin(\frac{ 2\pi jk}{n})}
        \end{aligned}
     \end{equation}

     As $\bx\sim_{iid} BG(\theta)$, we have $\abs{\sum_{j=0}^{n-1} x_{j+1} \cos(\frac{ 2\pi jk}{n})}$ is still sub-Gaussian with $\snorm{\abs{\sum_{j=0}^{n-1} x_{j+1} \cos(\frac{ 2\pi jk}{n})}}\leq C_b \sqrt{n}$ by Fact \ref{fact:BG to SG}. Similarly, $\snorm{\abs{\sum_{j=0}^{n-1} x_{j+1} \sin(\frac{ 2\pi jk}{n})}}\leq C_b \sqrt{n}$, so that we have
$\abs{\lambda_k}$ is sub-Gaussian with $\snorm{\abs{\lambda_k}}\leq \snorm{\abs{\sum_{j=0}^{n-1} x_{j+1} \cos(\frac{ 2\pi jk}{n})}}+\snorm{\abs{\sum_{j=0}^{n-1} x_{j+1} \sin(\frac{ 2\pi jk}{n})}}\leq C \sqrt{n}$.

    Then we obtain the tail bound for $\norm{\cC(\bx)}_{op}$ by Fact \ref{fact: tail bound of BG} as following:
    
    \begin{equation}
        \begin{aligned}
    \mbP{\norm{\cC(\bx)}_{op}\geq t}=\mbP{\max_{k\in[n]} \abs{\lambda_k}\geq t}\leq \sum_{k=1}^n \mbP{\abs{\lambda_k}\geq t}\leq 2n \exp\sbra{\frac{-t^2}{Cn}}\\
    \end{aligned}
\end{equation}

Utilizing the above tail bound, we derive the bound for the moments of circulant matrix $\norm{\cC(\bx)}_{op}^2$. WLOG, assuming $n\geq 2$,  we have
\begin{equation}
    \begin{aligned}
         \mathbb{E}(\norm{\cC(\bx)}_{op}^{2m})&=\int_0^\infty \mathbb{P}(\norm{\cC(\bx)}_{op}^{2m} >u) du\\
    &= \int_0^\infty \mathbb{P}(\norm{\cC(\bx)}_{op} >t)\cdot 2m t^{2m-1} dt \qquad (t=u^{1/2m})\\
    &\leq \int_0^{\sqrt{4C n\log(n)}} 1\cdot 2m t^{2m-1} dt +\int_{\sqrt{4C n\log(n)}}^\infty 2n\exp\sbra{\frac{-t^2}{Cn}}2m t^{2m-1} dt\\
    &\leq 2m\sbra{4Cn \log(n)}^m + \int_{\sqrt{4C n\log(n)}}^\infty \exp\sbra{\frac{-t^2}{2Cn}}2m t^{2m-1} dt
    \qquad  ( \exp\sbra{\frac{-t^2}{2Cn}}>2n\exp\sbra{\frac{-t^2}{Cn}})\\
    &\leq 2m\sbra{4Cn \log(n)}^m +\int_0^\infty \sbra{2Cn}^m \exp\sbra{-v^2}2m v^{2m-1} dv  \qquad (v=\frac{t}{\sqrt{2Cn}})\\
    &=2m \sbra{4Cn \log(n)}^m + \sbra{2Cn}^m 2m\cdot \Gamma(m)\\
    &=2m \sbra{4Cn \log(n)}^m + 2\sbra{2Cn}^m m!\\
    &\leq \frac{m!}{2} \sbra{C' n \log(n)}^m\\
    \end{aligned}
\end{equation}
\end{proof}

\begin{lemma} (Bound for gradient)\label{lemma:Bound for gradient}
    The tail bound for $\norm{\nabla_{\bw}\phi(\bm{0},\bI)}_2$ is
    \begin{equation}
        \mbP{\norm{\nabla_{\bw}\phi(\bm{0},\bI)}_2\geq t}\leq 2(n+1)\exp \sbra{\frac{-pt^2}{4n^3+2\sqrt{2}n^{3/2}t}}
    \end{equation}
\end{lemma}

\begin{proof}

We are going to derive the tail bound using moment-control Bernstein inequality \ref{lemma:vector bernstein}. As $\nabla_{\bw}\phi(\bm{0},\bI)=\frac{1}{p}\sum_{k=1}^p \nabla_{\bw} \psi_{\mu}\sbra{\cC(\bx^{(k)})\bh(\bm{0})}$, we need to bound the moments of $\norm{\nabla_{\bw} \psi_{\mu}\sbra{\cC(\bx)\bh(\bm{0})}}$. 
\begin{equation}
    \begin{aligned}
    \norm{ \nabla_{\bw} \psi_{\mu}\sbra{\cC(\bx^{(k)})\bh(\bm{0})}}
    &\leq \norm{\sum_{j=0}^{n-1}\nabla_{\bw} \psi_{\mu}\sbra{\cS_j(\hx^{(k)})^\top \bh(\bm{0})}}\\
    &= \norm{\sum_{j=0}^{n-1}\tanh\sbra{\frac{\cS_j(\hx^{(k)})_n}{\mu}}\cdot \mathcal{S}_j(\hx^{(k)})_{1:n-1}}\\
    &\leq \sum_{j=0}^{n-1} \norm{\mathcal{S}_j(\hx^{(k)})_{1:n-1}}_2
    \end{aligned}
\end{equation}
since $\abs{\tanh\sbra{\frac{\cS_j(\hx)_n}{\mu}}}\leq 1$. Then, we obtain
\begin{equation}
    \mbE{\norm{\nabla_{\bw} \psi_{\mu}\sbra{\cC(\bx)\bh(\bm{0})}}^m}\leq \mbE{\sbra{n\norm{\bx}}^m}\leq n^m \mathbb{E}_{\bx\in \gd{\bI}} \sbra{\sbra{n\norm{\bx}}^m} \leq m! \cdot n^{\frac{3m}{2}}
\end{equation}
using Lemma \ref{lemma: Moments bound for chi}.

We have $$\mathbb{E}\sbra{\nabla_{\bw}\phi(\bm{0},\bI)}=\mathbb{E}\sbra{\nabla_{\bw} \psi_{\mu}\sbra{\cC(\bx^{(k)})\bh(\bm{0})}}=0$$
Finally, we let $\sigma^2=(2n^3), R=\sqrt{2} n^{3/2}$ and complete the proof by Corrolary \ref{lemma:vector bernstein}.
\end{proof}

\begin{lemma} (Lipschitz for subsets) \label{lemma:Lipschitz for staying in subsets}
    For fixed $\bx$, and any $\bh,\bh'\in \cS_{\xi_0}^{n+}$ and for all $i\in[n-1]$ with $h_i,h_i'\neq 0, \frac{h_n^2}{h_i^2}<4,\frac{h_n'^2}{h_i'^2}<4$, we have
    \begin{equation}
        \begin{aligned}
            \abs{\tanh \sbra{\frac{\bx^\top \bh}{\mu}}-\tanh \sbra{\frac{\bx^\top \bh'}{\mu}}}&\leq \abs{\frac{\bx^\top\bh}{\mu}-\frac{\bx^\top\bh'}{\mu}} \leq \frac{1}{\mu}\norm{\bx}\norm{\bh-\bh'}_2 \\
            \abs{\tanh \sbra{\frac{\bx^\top \bh}{\mu}}}&\leq 1\\
            \abs{\sbra{\frac{x_i}{h_i}-\frac{x_n}{h_n}}-\sbra{\frac{x_i}{h'_i}-\frac{x_n}{h'_n}}}&\leq5n \norm{\bx}_\infty \norm{\bh-\bh'}\\
            \abs{\sbra{\frac{x_i}{h_i}-\frac{x_n}{h_n}}}&\leq 2\sqrt{n} \norm{\bx}_\infty
        \end{aligned}
    \end{equation}
\end{lemma}

\begin{proof}

For the third inequality, We have
\begin{equation}
    \begin{aligned}
        \abs{\sbra{\frac{x_i}{h_i}-\frac{x_n}{h_n}}-\sbra{\frac{x_i}{h'_i}-\frac{x_n}{h'_n}}}&\leq \abs{x_i}\abs{\frac{h_i-h'_i}{h_i h'_i}}+\abs{x_n}\abs{\frac{h_n-h'_n}{h_n h'_n}}\\
        &\leq 4n \norm{\bh-\bh'} \abs{x_i}+ n \norm{\bh-\bh'} \abs{x_n}\\
        &\leq 5n \norm{\bx}_\infty \norm{\bh-\bh'}
    \end{aligned}
\end{equation}
since $h_n\geq \frac{1}{\sqrt{n}}$ and $ \frac{h_n}{h_i}<2$.

The lefted inequalities are obtained by simple bound, $h_n\geq \frac{1}{\sqrt{n}}$ and Cauchy inequalities.

\end{proof}

\begin{lemma}\label{lemma: other1}
    For independent sequence of vectors $\{\bx_i \}_{i=1}^p\in\mathbb{R}^n$ with $\bx_i\sim_{iid} BG(\theta)$, $\theta\in (0,1/2)$, there exists a constant $C$, such that
    \begin{equation}
 \norm{\frac{1}{\theta np} \sum_{i=1}^p \cC(\bx_i)^\top \cC(\bx_i)-\bI}\leq C\sqrt{\frac{\log^2(n) \log(p)}{\theta^2 p}}
    \end{equation}
    with probability at least $1- 2n p^{-8}$
\end{lemma}
\begin{proof}
For convenient, let $\bV=\frac{1}{\theta np} \sum_{i=1}^p \cC(\bx_i)^\top \cC(\bx_i)$. We are going to derive the tail bound for the deviation between matrix $\bV$ and identity matrix $\bI$ using moment-control Bernstein's inequality in Lemma~\ref{lemma:matrix_bernstein}.
As $\bV=\frac{1}{\theta np} \sum_{k=1}^p \cC(\bx_k)^\top \cC(\bx_k)$ comes from $p$ independent matrixes with same distribution, we consider the moments bound for one component $\frac{1}{\theta n}\cC(\bx_i)^\top \cC(\bx_i)$ as following:

\begin{equation}
    \begin{aligned}
        \mathbb{E}\sbra{\mbra{\frac{1}{\theta n}  \cC(\bx_i)^\top \cC(\bx_i)}^m}& \preceq \frac{1}{\theta^m n^m}\mathbb{E}\sbra{ \norm{\cC(\bx_i)^\top \cC(\bx_i)}^m} \bI\\
        &= \frac{1}{\theta^m n^m}\mathbb{E}\sbra{ \norm{\cC(\bx_i)}^{2m}} \bI\\
        &\preceq  \frac{m!}{2} \sbra{\frac{4C\log(n)}{\theta}}^m \bI
    \end{aligned}
\end{equation}

where the last line comes from Lemma \ref{lemma:Operator norm of Circulant Matrix}. Finally, as we have $\mbE{\frac{1}{\theta np} \sum_{i=1}^p \cC(\bx_i)^\top \cC(\bx_i)}= \mbE{\frac{1}{\theta n} \cC(\bx)^\top \cC(\bx)}=\bI$, let $\sigma^2= \frac{16C^2 \log^2 (n)}{\theta^2}$, $R=\frac{4C \log(n)}{\theta}$, we have the tail bound
\begin{equation}\label{equ:F_i}
    \mathbb{P}\sbra{\norm{\frac{1}{\theta np} \sum_{i=1}^p \cC(\bx_i)^\top \cC(\bx_i)-\bI}\geq t} \leq %2n \exp\sbra{\frac{-pt^2}{18\cdot 16n^2+9\cdot 2nt}}\leq 
    2n \exp\sbra{\frac{-p\theta^2 t^2}{32C^2 \log^2 (n)+ 8C \log(n)\theta t}}.
\end{equation}
by Lemma \ref{lemma:matrix_bernstein}.

Setting $t=C\sqrt{\frac{\log^2(n)\log(p)}{\theta^2 p}}$, we complete the proof.

\end{proof}

\begin{lemma} (Integral form of Taylor Theorem) \label{integral Taylor}
    Let $f(\bx): \mathbb{R}^n \mapsto \mathbb{R}$ be a twice continutously diffenrentiable function, the for $\by\in\mathbb{R}^n$, we have
    \begin{equation}
        f(\bx-\eta \by)=f(\bx)- \left \langle \nabla f(\bx), \eta \by \right \rangle+ \eta^2\int_0^1 (1-s)\by^\top \nabla^2 f(\bx-s\eta\by) \by ds.
    \end{equation}
\end{lemma}

\begin{lemma}\label{lemma:Lipschitz for general case}

For independent sequence of vectors $\{\bx_i\in\mathbb{R}^n\}_{i=1}^p$ with $\bx_i\sim_{iid} BG(\theta)$ and any $\by\in\mathbb{R}^n$,
we have the bound and lipschitz property of gradient as:
    \begin{equation}
        \begin{aligned}
         \max_{i\in[p]} \norm{\tanh\sbra{ \frac{\cC(\bx_i) \cdot \bh}{\mu}} - \tanh\sbra{ \frac{\cC(\bx_i) \cdot \bh'}{\mu}} }&\leq \frac{1}{\mu} \max_{i\in[p]}\norm{\cC(\bx_i)}\norm{\bh-\bh'}_2.\\
         \norm{\tanh\sbra{ \frac{\by}{\mu}}  }&\leq \sqrt{n}
         \end{aligned}
    \end{equation}

For the lipschitz property of the Hessian, with probability at least $1-(np)^{-8}$, we have 
    \begin{equation}
        \begin{aligned}
            \sup_{i\in[p]}\frac{1}{\mu}\norm{\diag\mbra{1-\tanh^2\sbra{ \frac{\cC(\bx_i) \cdot \bh}{\mu}}} - \diag\mbra{1-\tanh^2\sbra{ \frac{\cC(\bx_i) \cdot \bh'}{\mu}}}   }_{op} &\leq \frac{C_d}{\mu^2}\norm{\bh-\bh'}_2 \sqrt{\log(np)}\\
            \norm{\frac{1}{\mu}\diag\mbra{1-\tanh^2\sbra{ \frac{\by}{\mu}}} }_{op} &\leq \frac{1}{\mu}.
        \end{aligned}
    \end{equation}
\end{lemma}

\begin{proof}
For the lipschitz property of gradient, we have for any $\bx_i$,
\begin{equation}
    \begin{aligned}
        \norm{\tanh\sbra{ \frac{\cC(\bx_i) \cdot \bh}{\mu}} - \tanh\sbra{ \frac{\cC(\bx_i) \cdot \bh'}{\mu}} }&=\mbra{\sum_{j=0}^{n-1} \abs{\tanh \sbra{\frac{\cS_j(\hx_i)^\top \bh}{\mu}}-\tanh \sbra{\frac{\cS_j(\hx_i)^\top \bh'}{\mu}}}^2   }^{1/2}\\
        &\leq \mbra{\sum_{j=0}^{n-1} \abs{\sbra{\frac{\cS_j(\hx_i)^\top \bh}{\mu}}-\sbra{\frac{\cS_j(\hx_i)^\top \bh'}{\mu}}}^2   }^{1/2}\\
        &\leq \frac{1}{\mu} \norm{\cC(\bx_i) \sbra{\bh-\bh' }  }_2\\
    \end{aligned}
\end{equation}
where the second line is obtained by Lemma \ref{lemma:loss_lipschitz}. Therefore, by the fact $\norm{\cC(\bx_i) \sbra{\bh-\bh'}}\leq \norm{\cC(\bx_i)}\cdot \norm{\bh-\bh'}$, we have
 \begin{equation}
         \max_{i\in[p]} \norm{\tanh\sbra{ \frac{\cC(\bx_i) \cdot \bh}{\mu}} - \tanh\sbra{ \frac{\cC(\bx_i) \cdot \bh'}{\mu}} }\leq \frac{1}{\mu} \max_{i\in[p]}\norm{\cC(\bx_i)}\norm{\bh-\bh'}_2.
\end{equation}

We also have
\begin{equation}
    \norm{\tanh\sbra{ \frac{\cC(\bx_i) \cdot \bh}{\mu}}}= \sqrt{\sum_{j=0}^{n-1}  \tanh^2\sbra{ \frac{\cS_j(\hx_i) \cdot \bh}{\mu}}}\leq n.
\end{equation}
as $\abs{\tanh(x)}\leq 1$.

For the lipschitz property of the Hessian, we have
\begin{equation}
    \begin{aligned}
         &\quad \frac{1}{\mu}\norm{\diag\mbra{1-\tanh^2\sbra{ \frac{\cC(\bx_i) \cdot \bh}{\mu}}} - \diag\mbra{1-\tanh^2\sbra{ \frac{\cC(\bx_i) \cdot \bh'}{\mu}}}   }_{op}\\
         &=\frac{1}{\mu}\abs{\mbra{1-\tanh^2\sbra{ \frac{\cC(\bx_i) \cdot \bh}{\mu}}}-\mbra{1-\tanh^2\sbra{ \frac{\cC(\bx_i) \cdot \bh'}{\mu}}}}_\infty\\
         &\leq \frac{2}{\mu^2} \norm{\cC(\bx_i)\sbra{\bh-\bh'}}_\infty\\
         &=\frac{2}{\mu^2} \max_{j\in[n]} \abs{\sbra{\bh-\bh'}^\top \cS_j(\hx_i)}
    \end{aligned}
\end{equation}
where the third line is obtained by Lemma \ref{lemma:loss_lipschitz}.

Then we turn to derive the bound for maximum of $\abs{\sbra{\bh-\bh'}^\top \cS_j(\hx_i)}$.
As $\cS_j(\hx_i)\sim_{iid} BG(\theta)$, we have $\snorm{\sbra{\bh-\bh'}^\top \cS_j(\hx_i) }\leq C_b \norm{\bh-\bh'}_2$ by Fact \ref{fact:BG to SG}, the property of Bernoulli-Gaussian vector. So we have the tail bound that
    \begin{equation}
        \mbP{\sup_{i\in[p]} \mbra{ \max_{j\in[n]} \abs{\sbra{\bh-\bh'}^\top \cS_j(\hx_i)} }\geq t}\leq 2np\exp \sbra{\frac{-t^2}{C_b^2\norm{\bh-\bh'}_2^2}},
    \end{equation}
thus, setting $t=C_d \norm{\bh-\bh'}\sqrt{\log(np)}$, we complete the proof.

\end{proof}
